# Supplementary material for: Legibot: Generating Legible Motions for Service Robots Using Cost-Based Local Planners
Source: arXiv:2404.05100 source file (2024-04-07)
Supplement: Supplementary file 1 [file appendix_legib_eq.tex]

In \cite{dragan2013legibility}, the legibility of a piece of a trajectory $\xi$ is defined
by estimating the most probable goal of the robot based on the observed trajectory $P(G|\xi_{S \to Q})$.
%To quantify the legibility of a robot's motion, we start from the legibility score proposed by Dragan et al. \cite{dragan2013legibility}
%which is based on the idea of minimizing the ambiguity of the robot's goal for the observers.
%This means, an observer should be able to predict the robot's goal with high confidence, as the robot moves.
%Here, we want to estimate $\mathcal{I}_L$ the most probable goal of the robot based on the observed trajectory:
%
%\begin{equation}
%    \label{eq:dragan3}
%    \mathcal{I}_L (\xi_{S \to Q}) = \arg \max_{G \in \mathcal{G}} P(G|\xi_{S \to Q})
%\end{equation}
%
%\noindent
%where $\xi_{S \to Q}$ is the observed trajectory from the start point $S$ to the query point $Q$,
%and $P(G|\xi_{S \to Q})$ is the probability of the robot's goal being $G$ given the observed trajectory $\xi_{S \to Q}$.
%
Using the Bayes' rule, it will be proportional to $P(\xi_{S \to Q}|G)$ and $P(G)$,
%and assuming a trajectory can be separated into two part,
where the first term can be written as below:

\begin{equation}
    \label{eq:dragan6}
    P(\xi_{S \to Q} | G) = \frac{P(\xi_{S \to Q}) \int_{\xi_{Q \to G}} P(\xi_{Q \to G})} {\int_{\xi_{S \to G}} P(\xi_{S \to G})}
\end{equation}

\noindent
Finally, using the suboptimality cost function $C(\xi)$ to estimate the probability of a trajectory, $P(G|\xi_{S \to Q})$ can be obtained.
Here, for the sake of simplicity to interpret the equation, we write the logarithmic form:

%\begin{equation}
%    \label{eq:dragan8}
%    P(G | \xi_{S \to Q}) = \frac{1}{Z} \frac{\exp \left(-C\left(\xi_{S \to Q}\right)-C\left(\xi^*_{Q \to G}\right)\right)}{\exp \left(-C\left(\xi^*_{S \to G}\right)\right)} P(G)
%\end{equation}
%
%\noindent
%where $Z$ is a normalization constant.
%\noindent
%You can follow the derivation of the above equation in the original paper \cite{dragan2013legibility}. % or Dragan's thesis \cite{dragan_thesis}.
%
%By applying the logarithmic transformation to Eq. \ref{eq:dragan8}, for the sake of simplicity, we can rewrite it as below:
%
\begin{equation}
    \label{eq:dragan8_log}
    \begin{split}
    & \log P(G | \xi_{S \to Q}) = \\
    & \log (P(G)/Z) + C(\xi^*_{S \to G}) - C(\xi_{S \to Q}) - C(\xi^*_{Q \to G})
    \end{split}
\end{equation}

\noindent
This equation implies the probability of the robot's goal being $G$ given $\xi_{S \to Q}$ depends on the following terms:
\begin{enumerate}[leftmargin=*]
    \item $P(G)/Z$: The prior probability of the robot's goal being $G$ in the observe's belief, normalized by factor $Z$.
                    $P(G)$ is usually set to a uniform distribution assuming the observers have no prior knowledge about the robot's goal.
    \item $C(\xi^*_{S \to G})$: is the suboptimality cost of the optimal trajectory $\xi^*_{S \to G}$, and is independent of the robot's decision.
    \item $C(\xi_{S \to Q})$: is the suboptimality cost of the observed trajectory $\xi_{S \to Q}$, and it does not depend on the robot's goal, and contributes equally to the probability of all the goals.
    \item $C(\xi^*_{Q \to G})$: is the suboptimality cost of the optimal trajectory $\xi^*_{Q \to G}$, and is the only term that can make the probability of the robot's actual goal being different from the probability of other goals.
\end{enumerate}

In \cite{dragan2013generating} the legibility score is defined as below, by introducing a descending function $f(t)$ which assigns higher weights to the initial parts of the trajectory:

\begin{equation}
    \label{eq:dragan9}
    \text { legibility }(\xi)=\frac{\int P\left(G^* \mid \xi_{S \rightarrow \xi(t)}\right) f(t) d t}{\int f(t) d t}
\end{equation}

\noindent
The authors suggest that Eq. (\ref{eq:dragan9}) can never reach to its maximum value of 1, in a finite space.
And they propose a trust region constraint on the optimization, to ensure the motion does not become too surprising or unpredictable to the observer.
Then, the problem will be reduced to finding a good value for a parameter $\beta$, using a user study.
Also in \cite{dragan2013legibility} this is handled by adding a regularizer that discourage increasing the path length.
$L(\xi) = legibility(\xi) - \lambda C(\xi)$
where $C(\xi)$ is the path length, and $\lambda$ is a constant.
